# Supplementary material for: Relaxometry and contrast-free cerebral microvascular quantification using balanced Steady-State Free Precession MR Fingerprinting
Source: arXiv:2411.03414 source file (2024-11-05)
Supplement: Supplementary file 1 [file Supp_Coudert_MRM_2024-30-38.pdf]

Relaxometry and contrast-free cerebral microvascular quantification  
using balanced Steady-State Free Precession MR Fingerprinting

Thomas Coudert | Aurélien Delphin | Antoine Barrier | Loïc Legris | Jan M Warnking | Laurent  
Lamalle | Mariya Doneva | Benjamin Lemasson | Emmanuel L Barbier | Thomas Christen

**SUPPLEMENTARY MATERIALS**

**Figure S1:** Examples of the effect of water diffusion on the signal shape simulated using the MRvF-bSSP sequence proposed in our method for  $T_1=1.6s$ ,  $T_2=0.2s$ ,  $B_1=0.7$ ,  $\delta f=5Hz$ ,  $SO_2=50\%$ ,  $VF=3\%$ ,  $R=5\mu m$  (left) and  $T_1=1.1s$ ,  $T_2=0.11s$ ,  $B_1=1.0$ ,  $\delta f=25Hz$ ,  $SO_2=80\%$ ,  $VF=5\%$ ,  $R=5\mu m$  (right).

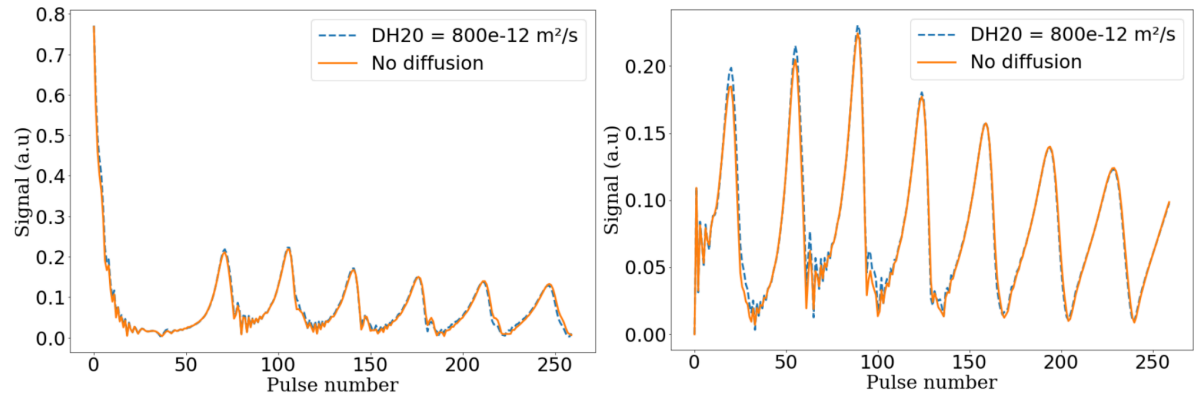

**Figure S2:** Simulation parameters for the three dictionaries presented in the Methods section.

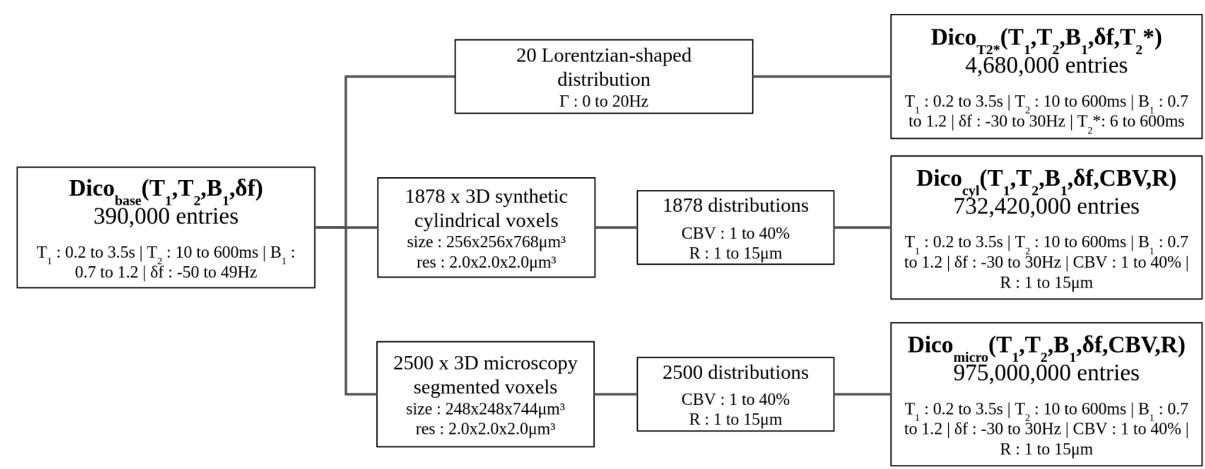

**Figure S3:** Intra-voxel frequency distribution for a synthetically generated voxel with cylindrical vessels, for  $SO_2=60\%$ ,  $CBV=5\%$ , and  $R=6\mu m$ . Each line corresponds to a different voxel size. Please note that the random position of the vessels slightly changes the distribution for the two voxels of the same  $SO_2$ ,  $CBV$ , and  $R$ . However, significant changes in the distributions appear when changing the size ratio between the different axes of the voxel, especially when modifying the X and Y ratios compared to the Z ratio when the magnetic field is oriented in the Z direction of the voxel.

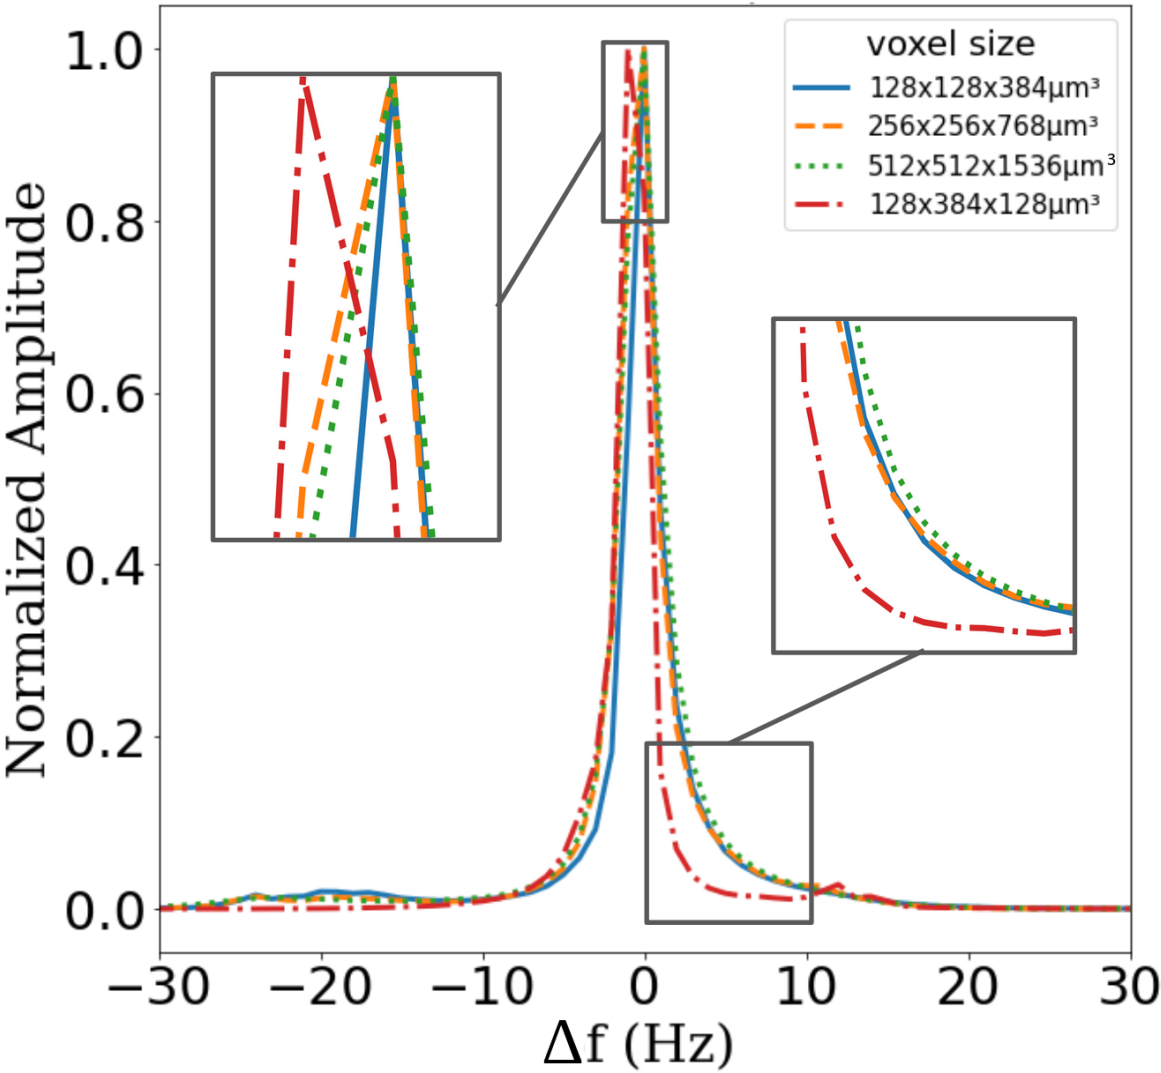

**Figure S4:** Intra-voxel frequency distributions computed from synthetic cylindrical voxel without (a) and with (b) the presence of USPIO contrast agent. Distributions are plotted after normalization to enhance figure readability.

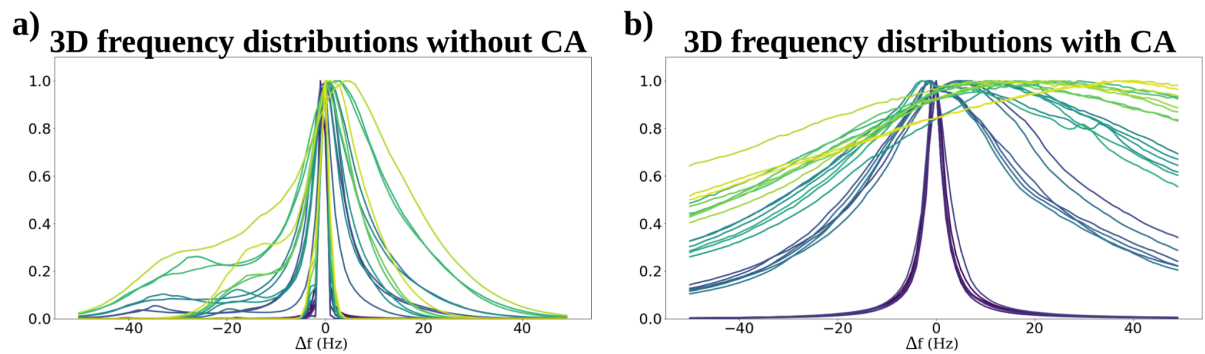

**Figure S5:** In vivo matched results of intra-voxel frequency distributions (associated with CBV and R values) in anatomic ROIs for one subject. SS=Sagittal sinus, WM=White Matter, GM=Grey Matter.

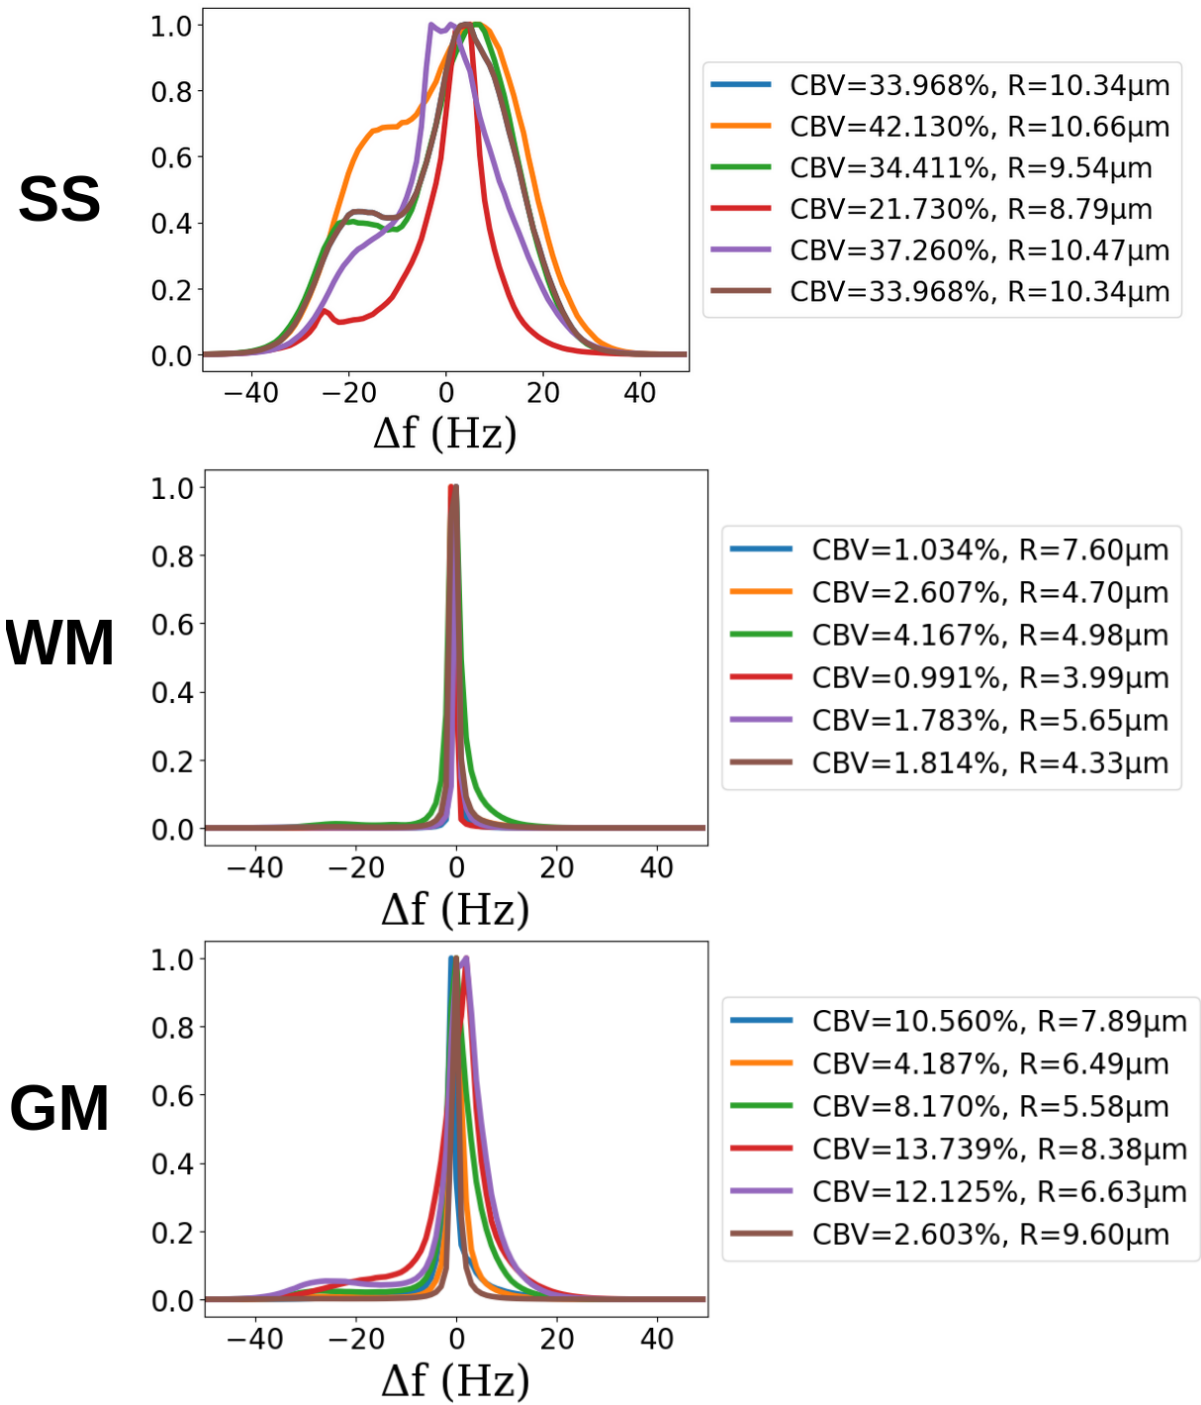

**Figure S6:** In vivo quantitative maps for the 6 healthy volunteers of the study.

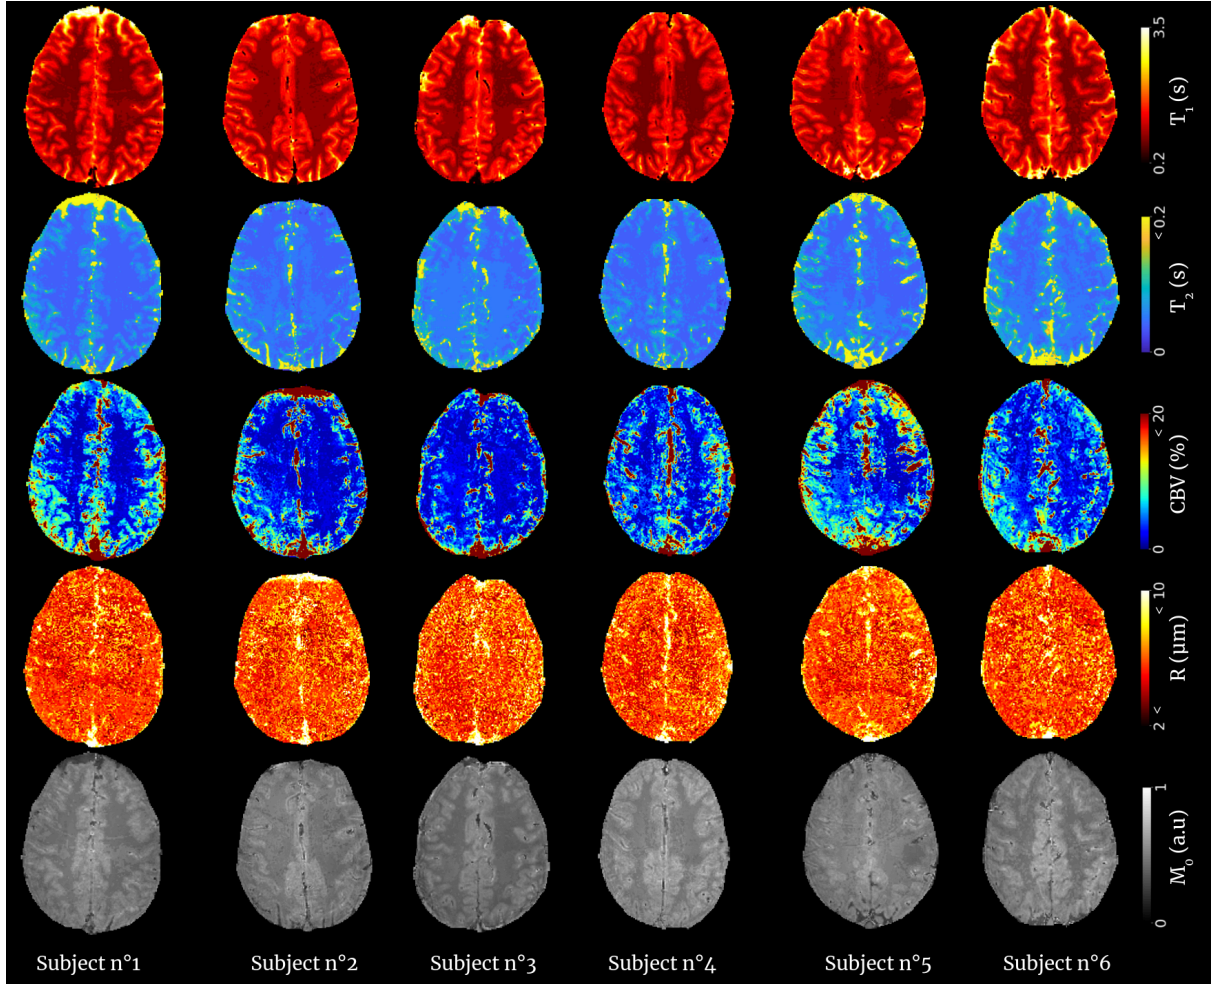

**Figure S7:** In vivo quantitative maps for one subject using the Lorentzian distribution for T2\* quantification. MRF dictionary was simulated without (a) and with (b) slice profile effects. Reference quantitative maps are shown below. Reference T1&T2 maps (c) were derived from an MRF dictionary matching using a standard MRF IR-FISP sequence. T2\* map (d) was computed by exponentially fitting an MGRE signal.

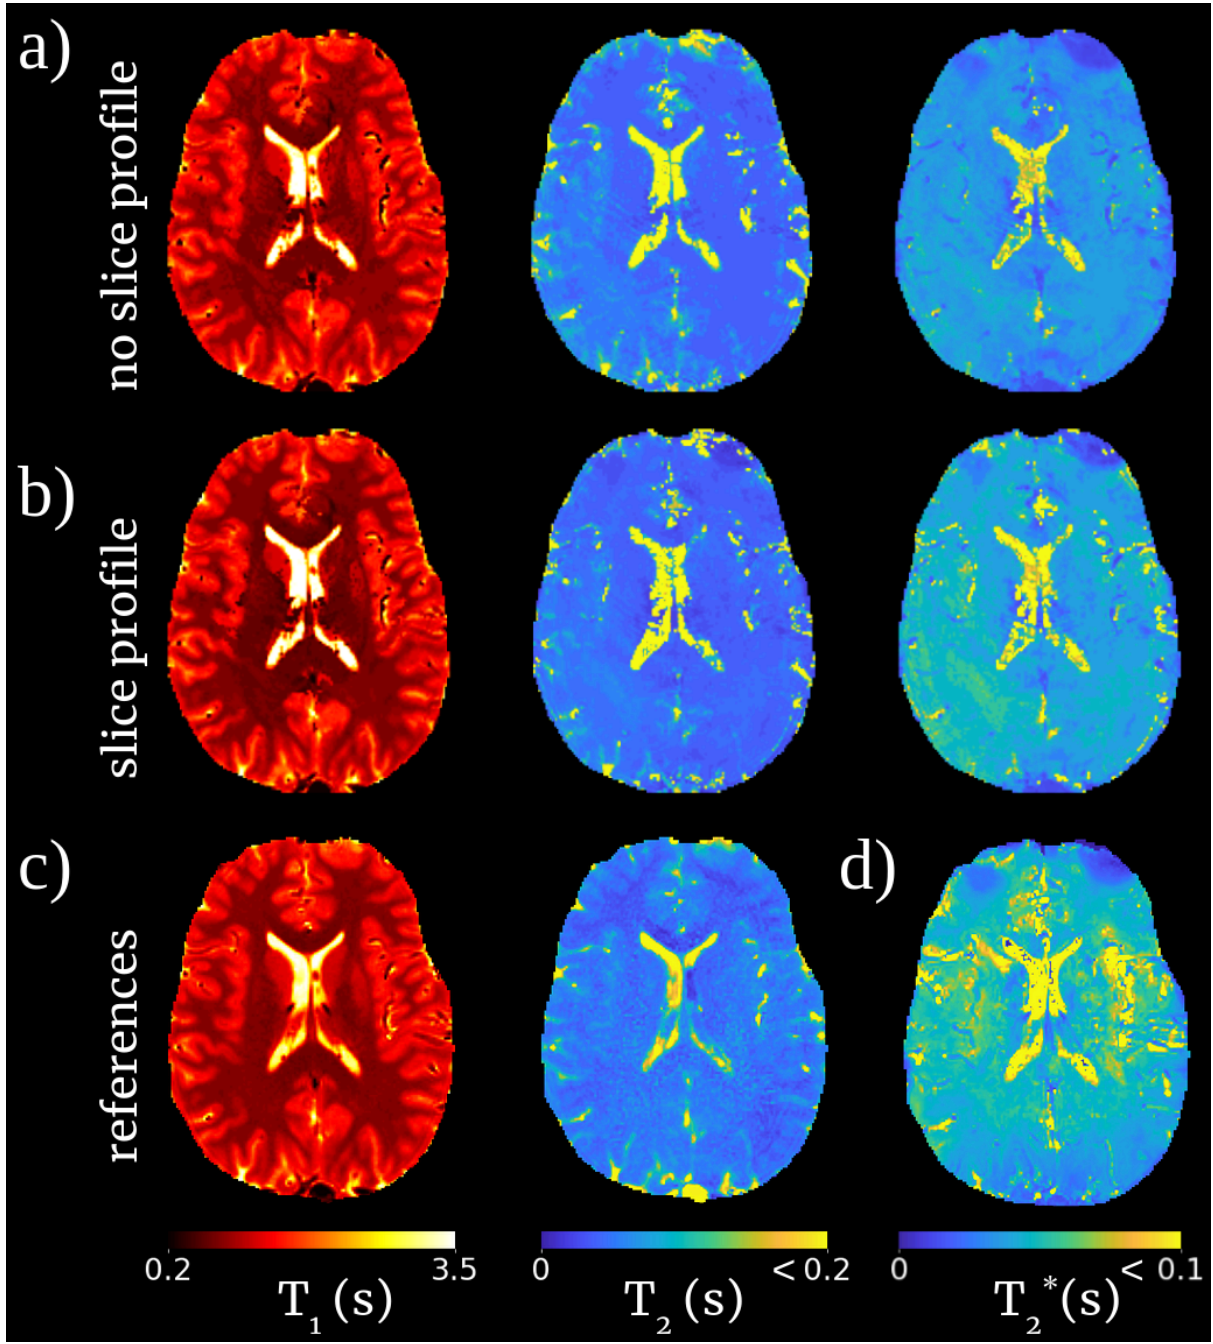

**Table S1:** ROIs values for T2\* MRF-bSSFP estimation with and without slice profile effect simulation.

| Parameter             | Tissue | No Slice Profile | Slice Profile | Reference |
|-----------------------|--------|------------------|---------------|-----------|
| T <sub>2</sub> * (ms) | WM     | 37 ± 2           | 47 ± 4        | 49 ± 2    |
|                       | GM     | 37 ± 2           | 51 ± 3        | 51 ± 2    |

T<sub>2</sub>\* reference values were exponentially fitting from a multi-echo GRE sequence.

**Partial-Volume MRF study of the MRF IR-FISP sequence**

For the high-resolution acquisition subject, a dictionary-based partial-volume analysis (PV-MRF, [Deshmane et al.](#)) was used to quantify myelin water fraction (MWF, see [Chen et al.](#)) based on the MRF IR-FISP sequence and a three-compartment model including myelin water (T1=130ms, T2=20ms), intracellular/extracellular water (T1=1300ms, T2=130ms) and free water (T1=4500ms, T2=500ms).

The below Figure S8 shows in vivo quantitative maps comparing high-resolution MRvF bSSFP estimate of external “B<sub>0</sub> gradient” and a partial-volume MRF IR-FISP estimate of Myelin Water Fraction.

Interestingly, the new B<sub>0</sub> gradient map presents spatial similarities with the myelin water fraction map as the highest B<sub>0</sub> gradient values are mainly localized in the white matter region of the brain.

**Figure S8:** In vivo quantitative maps comparing high-resolution MRvF bSSFP estimate of external “B<sub>0</sub> gradient” and a partial-volume MRF IR-FISP estimate of Myelin Water Fraction

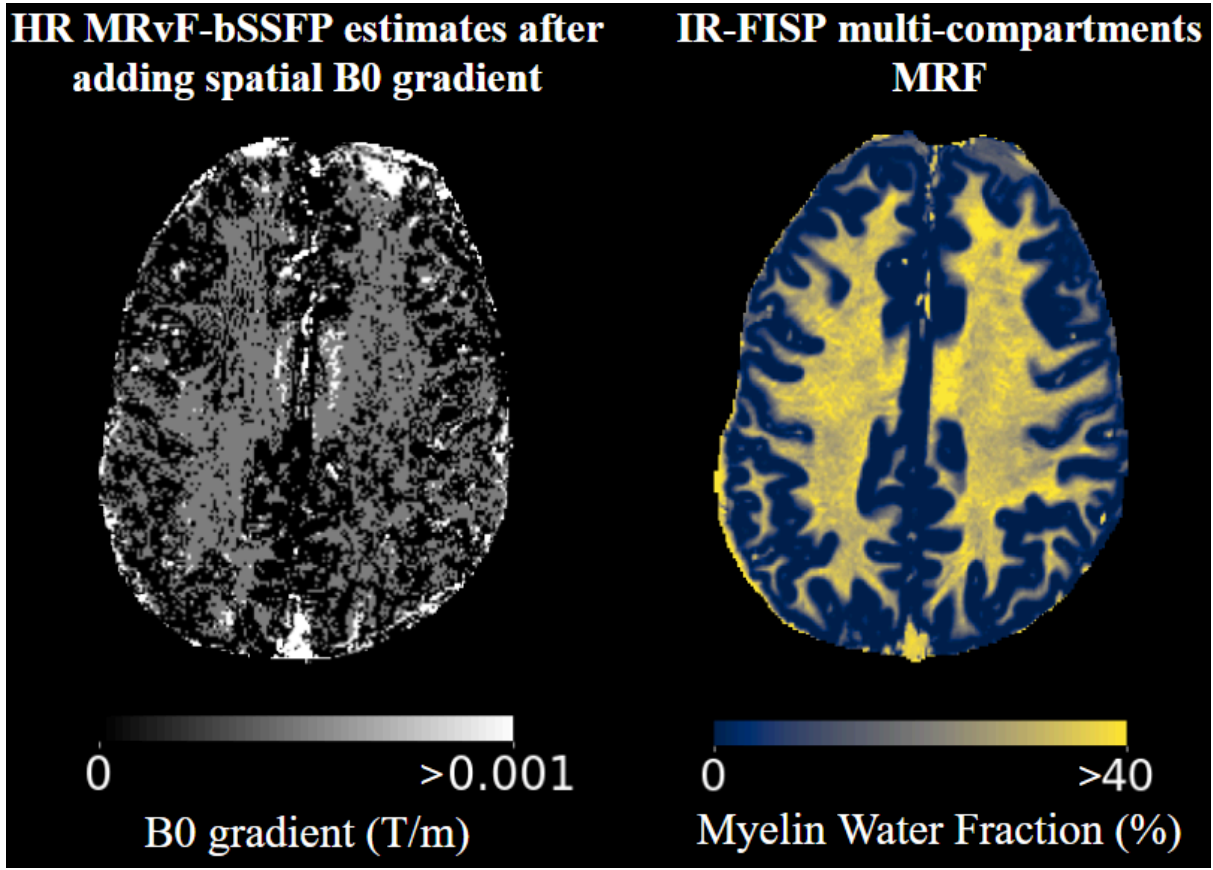

Deshmane A, Badve C, Rogers M, et al. Tissue mapping in brain tumors with partial volume magnetic resonance fingerprinting (PV-MRF). In: *Proceedings from the 23th Annual Meeting of ISMRM, Toronto.2015*

Chen Y, Chen MH, Baluyot KR, et al. MR fingerprinting enables quantitative measures of brain tissue relaxation times and myelin water fraction in the first five years of life. *NeuroImage*. 2019;186:782-793.
